# Supplementary material for: Procedural Multiscale Geometry Modeling using Implicit Functions
Source: arXiv:2504.09553 source file (2025-04-13)
Supplement: Supplementary file 1 [file future_work.tex]

\section{Discussion and Future work}
There are several exciting future directions for this research. One potential avenue is to enhance the current framework by incorporating wave optics-based simulations to capture diffraction effects. Additionally, the inclusion of polarization and fluorescence could provide more depth to the analysis.

Another intriguing direction involves analyzing an input image of a particle cloud from a particular slice of a volume or a macroscopic rendering of the particulate material. In this case, we could extract particle size distributions and volume fractions to model the entire volume based on a specific patch or image of the material. This approach focuses on deriving particle statistics from the input data to reconstruct the complete volume. Techniques such as static light scattering, dynamic light scattering, or laser diffraction can be employed to measure these particle size distributions. Furthermore, neural network-based methods can aid in determining particle statistics from the available data on size distributions and volume fractions.

In this work, we focused solely on material appearance modeling utilizing multiscale geometry through SDFS. However, in the future, we plan to optimize various material properties, including thermal, mechanical, electrical, and chemical characteristics, in relation to the corresponding geometry at different length scales.

Another possible area of exploration is the generation of particle flow effects to simulate fluid motion, including the modeling of Brownian motion of particles.

% Reconstrution
In this paper, we explore some optimization strategies to reconstruct the geometric patterns from direct parameter fitting, image exemplars or incomplete volumetric information as a proof of concept with synthetic data. For future work, it would be interesting to reconstruct real microstructures using SEM/TEM images or microCT volumes. Reconstruction from SEM/TEM images would require to adapt the synthesis module to at least roughly mimic the appearance under an electronic microscope or ideally a suitable Monte Carlo simulator like Nebula. One possibility to handle the inability of our current reconstruction approaches to handle high-dimensional problems is to apply a surrogate loss~\cite{fischer2024zerograds} or explore neural network-based optimization techniques tailored for procedural models.   
