# Supplementary material for: Procedural Multiscale Geometry Modeling using Implicit Functions
Source: arXiv:2504.09553 source file (2025-04-13)
Supplement: Supplementary file 2 [file rendering.tex]

\section{Multiscale Geometry Rendering} \label{sec:st}

We use conventional ray tracing methods when we render particulate geometry bounded by a triangle mesh. The sign of particulate material SDF \( d_g \) at the surface indicates whether the ray interacts with the particles' material or the host medium. Our approach focuses on the surfaces of light-scattering many particles, giving the flexibility to use only surface shaders along with volume absorption~\cite{pharr2023physically}. One important aspect is that this choice is not a limitation of our method, but it highlights our capability to model particle geometry and render light scattering volumes using straightforward surface shaders.

We need to find the next surface intersection when once the path is in mesoscale geometry; we start by storing the sign of the first SDF and apply a minimum distance to prevent locating the ray's origin as the intersection point. Following the methodology of Hart's sphere tracing~\cite{hart1996sphere}, we proceed along the ray by utilizing the value of $d_g$ multiplied by the initial sign, which facilitates tracing through transparent particles. The normal vector is then employed for surface shading at a surface intersection point; we calculate the gradient of the SDF using central differences.

To terminate paths probabilistically, we implement a Russian roulette technique that is based on absorption occurring at a diffuse particle surface or through volume absorption between surfaces. Additionally, we establish a maximum trace depth, at which point we return black if it is exceeded. When determining the maximum trace depth for a scene, we start with an initial rendering with a low value of the maximum trace depth. This approach can result in the rendered material appearing darker due to early path termination. We then incrementally raise the maximum trace depth until the brightness of the rendered material stabilizes. Figure~\ref{fig:clustersizeintensity} illustrates the trace depth for various particle clouds with distinct parameters.

%One of the main advantages of our method, as compared with statistical methods based on scattering properties, is that our simple rendering pipeline works for all types of particles, from spherical to non-spherical. If we compute scattering properties using Lorenz-Mie theory, the distribution of the scattered light is only accurate for spherical particles. Computing scattering properties for non-spherical particles is a complicated task.

In general, we divide 
$d_g$ by the greatest magnitude of the gradient to ensure that the functions represent signed distance despite potentially being transformed to a non-Euclidean domain. We list some rules that we follow when performing affine transformations on point a $\bm{p}$ in the supplemental material for various Lipschitz bounds used for the affine transformations.
