# Supplementary material for: Procedural Multiscale Geometry Modeling using Implicit Functions
Source: arXiv:2504.09553 source file (2025-04-13)
Supplement: Supplementary file 5 [file related_work.tex]

\section{Related Work} \label{sec:related}

A particulate material can be represented by distributing particles across various points in a given space. These points can be utilized to influence the coloration of textures near each point~\cite{schachter1979random}, to render the particles as images~\cite{van1991spot,dischler2002texture}, or to connect the particles into a cohesive implicit surface~\cite{ricci1973constructive}. This approach results in a volume that captures the microgeometry of the particulate material. In the following sections, we will explore related research on modeling particulate materials, with an emphasis on procedural methods for defining implicit surfaces.

\subsection{Procedural Modeling of Particulate Materials}

Modeling particulate materials often involves procedural color variation. The bombing method~\cite{schachter1979random} distributes color bubbles, later adapted for 3D textures by Peachey~\cite{peachey1985solid}, storing bubble properties in a table for efficient lookup. This eliminates the need for surface parametrization in 2D textures.

Sparse convolution noise~\cite{lewis1984texture,lewis1989algorithms} translates point distributions into particulate color variations using a convolution kernel. Efficient generation methods for kernels with compact support~\cite{frisvad2007fast,luongo2020microstructure} employ space-filling arrangements of randomly positioned impulses, simplifying neighbor identification. We use this approach to create a space-filling particle distribution within a bounding sphere radius. Sparse convolution with Gabor noise kernels~\cite{lagae2009procedural} can be used to generate high-quality surface-level textures that are spectrally controlled. In this framework, we efficiently generate high-quality volumetric hypertextures using space-filling implicit object distributions.  Stolte~\cite{1003534} presented a method for efficiently filling space and voxelizing infinite implicit objects using recursive subdivision algorithms, which work best for repetitive structures and capture intricate details, such as cyclical surfaces.

Hypertexture~\cite{perlin1989hypertexture} extends color variation to density variations in a volume, enabling procedural surface rendering via ray marching~\cite{tuy1984direct,kajiya1984ray}. Worley~\cite{worley1996cellular} demonstrated that distances to nearest points effectively model surface irregularities in particulate materials. We apply this to transform our particle distribution into an SDF for physically based rendering.

Stereology estimates 3D particle number density from 2D exemplars, aiding tileable color variation in particulate materials~\cite{jagnow2004stereological,shu2014efficient}. The Worley method~\cite{dorsey1999modeling,soulie2007modeling} generates compact particle aggregates using a precomputed Poisson point distribution. Randomized particle instantiation within a volumetric tile disrupts tiling periodicity~\cite{meng2015multi}, while space-filling point distributions eliminate the need for tiling or precomputation~\cite{baerentzen2023curl}. We leverage this to create spatially variable particulate materials with an SDF representation.

Radial basis functions can encode color and SDF from 2D reference images~\cite{qian2023vector}. Unlike these localized precomputed variations, our approach provides functional shape modeling tools that operate throughout space, maintaining a fully space-filling SDF.

\subsection{Signed Distance Field Modeling and Rendering} 
Ricci~\cite{ricci1973constructive} defines solid surfaces using level sets within a distance field, employing $\max$ and $\min$ for union and intersection. Hart et al.\cite{hart1989ray} optimized rendering for such implicit objects, leading to sphere tracing\cite{hart1993sphere, hart1996sphere}, now widely used for rendering SDF-based objects. We leverage sphere tracing for Monte Carlo ray tracing of microgeometries.

Function-based representation of objects, along with the relations and operations defined by Pasko~\cite{pasko1995function}, has been used for blending, offsetting, and morphing geometric shapes and objects. SDFs enable Boolean operations, surface offsets, and blending via interpolation~\cite{payne1992distance}. Our particulate SDF modeling integrates these methods with spatially varying offsets. While SDFs can also model layered solids~\cite{cutler2002procedural}.

Precomputed SDFs benefit from adaptive grids for scalability~\cite{frisken2000adaptively}. Sparse voxel octrees improve multi-scale representation and interpolation~\cite{heitz2012representing}, while displacement fields reduce voxelization artifacts~\cite{brunton2021displaced}. Our procedural approach avoids voxelization artifacts and precomputation constraints, ensuring smooth scale transitions, though high sample counts are needed for antialiased rendering. Adaptive ray marching~\cite{morrical2019efficient, wu2022real} improves the efficiency of the sphere tracing method. We extend it to multiscale geometry modeling with adaptive grids, where varying grid scales in different volume regions require adaptive bounds (or stepping) for better performance than fixed-length steps. We used longer steps in coarse grid resolution and shorter steps in fine grid resolution adaptively.

ShaderToy provides procedural SDF modeling resources~\cite{jeremias2014shadertoy} (\href{https://www.shadertoy.com/}{https://www.shadertoy.com/}), while Takikawa et al.~\cite{takikawa2022dataset} offer optimized SDF functions. In our work, an SDF-defined macroscopic surface influences the size, shape, and density of contained particles.

\subsection{Simulation-based Particulate Materials}
Particle simulation offers an alternative to point distribution for generating particulate materials. Discrete element methods simulate particle motion and interactions~\cite{bell2005particle,zingsheim2024learning}, even for arbitrarily shaped particles using SDFs~\cite{lai2022signed}. However, managing large particle counts efficiently remains a challenge. Our on-the-fly particle generation can overcome this. Continuum-based modeling~\cite{narain2010free} could enable consistent particulate generation within a medium, presenting an interesting future direction.

Other physically-based simulations~\cite{zhao2023role} produce realistic particulate materials, such as in bread-making~\cite{baravalle2015procedural}, but require substantial pre-computation, memory, and resolution constraints.

Additionally, other physically-based simulation techniques can yield impressive results in particulate materials~\cite{zhao2023role}, such as in simulations of bread-making~\cite{baravalle2015procedural}. However, these methods often demand substantial pre-computation and memory usage, along with constraints regarding material extent and resolution.

\subsection{Neural-based Techniques}

Perlin noise~\cite{perlin1985image,perlin2002improving} combined with an encoder-decoder neural network can generate realistic 3D textures from 2D references~\cite{henzler2020learning}. Implicit periodic field networks use periodic encoding in MLPs to model particulate materials~\cite{chen2022exemplar}, but their reliance on precomputed 3D subvolumes makes them impractical for large-scale rendering.

A volumetric shell approach with material texture patches~\cite{kajiya1989rendering} can be enhanced using neural techniques~\cite{baatz2022nerf,kuznetsov2022rendering,diolatzis2023mesogan,huang2023nerf}. Unlike these methods, we provide an exact mesoscale geometry representation, which is essential for applications like transparent particles (e.g., air bubbles in ice). Generative models for spatially varying noise~\cite{maesumi2024one} are limited to surface noise, while learning volumetric noise remains challenging. Our work explores SDF-based volume reconstruction, enabling full-volume reconstruction from examples.

\subsection{Miscellaneous Methods}

 Hypervolume model~\cite{pasko2001constructive} explores volume representation using functional representations (FRep) with attributes, generating hypervolumes via constructive tree structures and blending operations. Inspired by the hypertexture mechanism, we developed a framework that dynamically generates spatially varying microstructures using implicit functions and CSG operations.

Volume perturbations~\cite{kniss2002interactive} capture high-frequency details for realistic material appearance, while generalized displacement maps~\cite{wang2004generalized} render non-height-field mesoscale structures. We employ perturbations to enhance microgeometry details in volume rendering.

Periodic surface modeling~\cite{wang2007periodic,lu2022structural} with triply periodic minimal surfaces (TPMS) enables intricate topological patterns across scales, including composite metamaterials. Leveraging trigonometric functions, we generate seamless multiscale microstructures with minimal parameters and computation.

Geometry textures~\cite{toledo2008geometry} and volumetric spot noise~\cite{turkay2016volumetric} synthesize surface details but are limited to surfaces. MesoGen~\cite{michel2023mesogen} tiles mesoscale patterns aperiodically on meshes. Unlike these, our framework uses implicit functions to generate spatially varying infinite microstructures inside volumes.

Porous material modeling~\cite{baravalle2017realistic} employs particle systems and procedural Voronoi foams~\cite{martinez2016procedural} for additive manufacturing but is restricted to porous structures. Point distributions~\cite{sahbaei2018implicit,baerentzen2023curl} create convex, blob-like porous microstructures but lack spatial variation. We introduce agglomeration to generate complex, curvy, laminar, and fibrous microstructures, enabling mixed media, multiscale properties, and regionally varied packing densities.
